# Supplementary material for: Belief Propagation with Quantum Messages for Quantum-Enhanced Classical Communications
Source: arXiv:2003.04356 ancillary file (2021-05-07)
Supplement: Supplementary file 1 [file supplementary_material.pdf]

# Supplementary Material for "Belief Propagation with Quantum Messages for Quantum-Enhanced Classical Communications"


Narayanan Rengaswamy,[1,*] Kaushik P. Seshadreesan,[2,†] Saikat Guha,[2,‡] and Henry D. Pfister[3,§]

[1]*Department of Electrical and Computer Engineering, University of Arizona, Tucson, Arizona 85721, USA*

[2]*College of Optical Sciences, University of Arizona, Tucson, Arizona 85721, USA*

[3]*Department of Electrical and Computer Engineering, Duke University, Durham, North Carolina 27708, USA*



(Dated: April 23, 2021)


## SUPPLEMENTARY METHODS

### Supplementary Note 1: Decoding Linear Codes Using BP

An $[n, k, d]$ binary linear code $\mathcal{C}$ can be defined by a binary parity-check matrix $H$ as follows:

$$\mathcal{C} \coloneqq \{\underline{x} \in \{0,1\}^n \colon H\underline{x}^T = \underline{0}^T,\ H \in \{0,1\}^{(n-k)\times n}\}. \tag{1}$$

Such a code encodes $k$ message bits into $n$ code bits, and the minimum Hamming weight of any codeword $\underline{x} \in \mathcal{C}$ is $d$. Consider the $[5, 3, 2]$ code, which we still denote as $\mathcal{C}$, defined by

$$H \coloneqq \begin{bmatrix} 1 & 1 & 1 & 0 & 0 \\ 1 & 0 & 0 & 1 & 1 \end{bmatrix}. \tag{2}$$

A factor graph (FG) for a linear code is a bipartite graph where the bits (variables) are represented by circle nodes and the checks (factors) are represented by square nodes. The FG representation of (the above definition of) $\mathcal{C}$ is as shown in Fig. 1 (of the main text), where $c_1$ and $c_2$ represent the two parity checks on the 5 bits of each codeword in $\mathcal{C}$. Observe that every linear code has multiple associated parity-check matrices, each of which forms a generator matrix for its dual code. Hence, the FG representation of a code depends on the chosen parity-check matrix.

A discrete memoryless channel is represented as $W$ and is defined by the channel transition probability matrix $W(y|x) \coloneqq \mathbb{P}[Y = y|X = x]$, which represents the probability of observing $y \in \mathcal{Y}$ at the output of the channel when its input was $x \in \mathcal{X}$. Here, $\mathcal{X}$ and $\mathcal{Y}$ represent the input and output alphabets of the channel, respectively. A well-known example for such a channel is the binary symmetric channel (BSC). For the BSC, $\mathcal{Y} = \{0, 1\} = \mathcal{X}$ and the transition matrix is defined as

$$W^{\mathrm{BSC}} \coloneqq \begin{bmatrix} 1-p & p \\ p & 1-p \end{bmatrix}, \tag{3}$$

where the $(i, j)$-th entry is $W^{\mathrm{BSC}}(y = j|x = i)$ and $0 \le p \le 0.5$. The FG in Fig. 1 (of the main text) shows the channel $W_k$ associated with each bit $k$ as a separate factor node that provides the channel transition probability value for the observed output $y_k$ for input $x_k = 0$ (and $x_k = 1$). This description is not limited to BSCs but we do assume that all bits go through the same channel, i.e., $W_k = W$ for all $k$.

Given the channel output vector, $\underline{y}$, the decoder tries to determine the codeword $\underline{x} \in \mathcal{C}$ that was actually sent at the input. The block maximum-a-posteriori (MAP) decoder calculates the posterior probability for each codeword in the code, given $\underline{y}$, and chooses the codeword with the maximum value. This is the optimal decoder in terms of block error rate. For the example 5-bit code $\mathcal{C}$, when all codewords are transmitted with equal probability, it calculates

$$p(\underline{x}|\underline{y}) = \frac{p(\underline{y}|\underline{x}) \cdot p(\underline{x})}{\sum_{\underline{x}\in\{0,1\}^5} p(\underline{y}|\underline{x}) \cdot p(\underline{x})} \tag{4}$$

---


* narayananr@arizona.edu, corresponding author; most of this work was done when he was with the Department of Electrical and Computer Engineering, Duke University, Durham, North Carolina 27708, USA

† kaushiksesh@email.arizona.edu, corresponding author

‡ saikat@optics.arizona.edu

§ henry.pfister@duke.edu

$$= \frac{\prod_{k=1}^{5} W(y_k|x_k) \cdot \mathbb{P}[\underline{x} \in \mathcal{C}]}{p(\underline{y})} \tag{5}$$

$$\propto \prod_{k=1}^{5} W(y_k|x_k) \cdot [\mathbb{I}(x_1 \oplus x_2 \oplus x_3 = 0)\mathbb{I}(x_1 \oplus x_4 \oplus x_5 = 0)] \tag{6}$$

$$= W(y_1|x_1) \cdot [\mathbb{I}(x_1 \oplus x_2 \oplus x_3 = 0)W(y_2|x_2)W(y_3|x_3)] \cdot [\mathbb{I}(x_1 \oplus x_4 \oplus x_5 = 0)W(y_4|x_4)W(y_5|x_5)], \tag{7}$$

$$\hat{\underline{x}}^{\mathrm{MAP}} := \underset{\underline{x} \in \{0,1\}^5}{\operatorname{argmax}} \; p(\underline{x}|\underline{y}), \tag{8}$$

where the constant of proportionality in (6) is independent of $\underline{x}$. While the complexity of the described method grows exponentially with the code dimension $k$, it can be reduced when the code's factor graph is a tree [1]. A related approach is the bit-MAP decoder which marginalizes the above joint posterior for each bit and makes a decision bit-wise. Hence, to decode bit 1, the bit-MAP decoder computes

$$\hat{x_1}^{\mathrm{MAP}} := \underset{x_1 \in \{0,1\}}{\operatorname{argmax}} \sum_{x_2,x_3,x_4,x_5 \in \{0,1\}^4} p(\underline{x}|\underline{y}) \tag{9}$$

$$= \underset{x_1 \in \{0,1\}}{\operatorname{argmax}} \left\{ W(y_1|x_1) \cdot \left[ \sum_{x_2,x_3 \in \{0,1\}^2} \mathbb{I}(x_1 \oplus x_2 \oplus x_3 = 0)W(y_2|x_2)W(y_3|x_3) \right] \cdot \left[ \sum_{x_4,x_5 \in \{0,1\}^2} \mathbb{I}(x_1 \oplus x_4 \oplus x_5 = 0)W(y_4|x_4)W(y_5|x_5) \right] \right\}. \tag{10}$$

Even though marginalizing a general joint probability distribution can have exponential complexity in the number of involved variables, the idea of BP is that this can be done efficiently when the code's factor graph is a tree and the factor nodes (FNs) have bounded degree [1]. For the example 5-bit code above, the tree FG allows one to use the distributive property of addition over multiplication and compute the sums involved in the two square brackets separately. Then the results can be pooled in one final step that takes their product and multiplies the result with $W(y_1|x_1)$. This is exactly BP on this FG, since the two local sums can be interpreted as "local beliefs" about the variable $x_1$ that are propagated to be combined with the "belief" from the channel observation $y_1$.

Formally, the BP algorithm is initialized by setting the local channel factors $W_k = W(y_k|x_k)$ based on the observations $y_k$ for both $x_k = 0$ and $x_k = 1$. Then, the variables $x_k$ simply pass on the message $(W(y_k|x_k = 0), W(y_k|x_k = 1))$ to their associated factor node(s). In the first half-iteration of BP involving the FN update, the factors $c_a$ calculate the "local belief" $\sum_{x_i \in \{0,1\}:\, i \in \partial a \setminus \{1\}} \mathbb{I}(\oplus_i x_i = x_1) \prod_i W(y_i|x_i)$ for both $x_1 = 0$ and $x_1 = 1$, where $\partial a$ represents the indices of the set of variables attached to the factor $c_a, a \in \{1, 2\}$. In the next half-iteration of BP involving the variable node (VN) update, the VN $x_1$ combines all incoming local beliefs (including $W(y_1|x_1)$) by taking their product and renormalizing the result to make it the exact posterior marginal distribution for $x_1$. Since this example has a tree FG, this completes BP for decoding the bit $x_1$. A similar procedure can be executed for the other variables as well, and the whole scheme can be combined into a parallel BP schedule to compute marginals for all variables simultaneously. If the FG is not a tree, then one usually runs BP for multiple iterations and uses the resulting estimates. It is also typical to choose the BP messages to be log-likelihood ratios $\log \frac{W(y_k|x_k=0)}{W(y_k|x_k=1)}$ in order to simplify implementation, but this is not relevant for this paper.

## Supplementary Note 2: Induced Channels in BP

It is very convenient to represent the operations performed by BP at each FN and VN abstractly as "local inference" over a "locally induced channel". For convenience, we consider a VN that is attached to exactly two FNs since a degree-$d$ VN can always be analyzed by sequentially merging two attached edges at a time. Supplementary Figure 1 illustrates this process for a VN.

In Supplementary Figure 1, all VNs other than $x$ that are connected to $c_1$ and $c_2$ can be combined into the VNs $y$ and $z$, respectively. The VNs $y$ and $z$ represent independent observations of the variable $x$ through the induced channels $W$ and $W'$, respectively. Note that this independence occurs precisely when the full FG is a tree. The channel $W$ (respectively $W'$) represents the conditional probability of all VNs in the subtree rooted at $c_1$ (respectively $c_2$) given $x$. The two induced channels can be combined into a single channel $W \circledast W'$ whose outputs are the concatenation of $y$ and $z$. The transition probabilities of this channel are

$$[W \circledast W'](y, z|x) = W(y|x) \cdot W'(z|x, y) \tag{11}$$

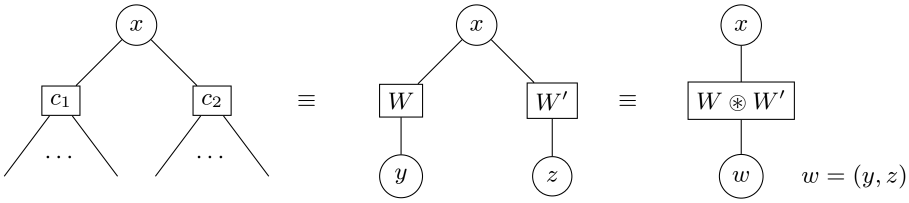


Supplementary Figure 1: Channel combining at a VN using the induced channels at the node.

$$= W(y|x) \cdot W'(z|x). \tag{12}$$

This is called the variable node convolution of two channels. Hence, the VN update operation of BP is simply performing local inference over the local channel $W \circledast W'$ i.e., calculating the local posterior for $x$ given $(y, z)$.

Similarly, at a (degree-3) FN we have a single input $x$ "splitting" into two outputs $u$ and $v$ (since they sum to $x$), whose independent observations through the underlying physical channel, as well as the remaining part of the FG, are obtained as $y$ and $z$. Then we have only two possibilities, either $u = x$ and $v = 0$ or $u = x \oplus 1$ and $v = 1$, and both of them are equally likely. Note that this is due to linearity of the code and holds under the assumption that the code does not have a trivial bit position where all codewords take the value 0. Hence, the factor node convolution of two channels $W$ and $W'$ is given by

$$[W \boxast W'](y, z|x) = \frac{1}{2}W(y|u = x) \cdot W'(z|v = 0) + \frac{1}{2}W(y|u = x \oplus 1) \cdot W'(z|v = 1) \tag{13}$$

$$= \frac{1}{2}W(y|x) \cdot W'(z|0) + \frac{1}{2}W(y|x \oplus 1) \cdot W'(z|1). \tag{14}$$

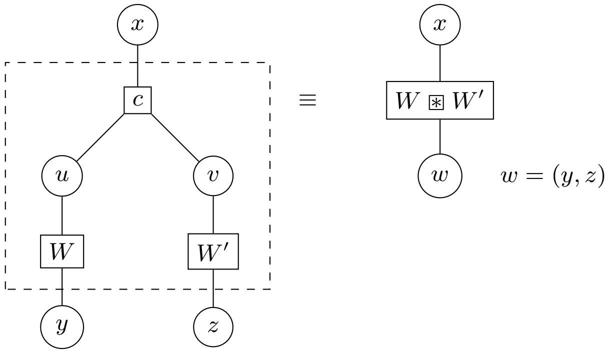


Supplementary Figure 2: Channel combining at a FN using the induced channels at the node.

We can perform a quick calculation using the FN update operation of BP to verify that BP is indeed performing local inference on this locally induced channel. In Fig. 1 (of the main text), consider the BP update at the FN $c_1$. We observe that

$$\sum_{x_2,x_3 \in \{0,1\}^2} \mathbb{I}(x_1 \oplus x_2 \oplus x_3 = 0) W(y_2|x_2) W(y_3|x_3)$$

$$= \sum_{x_2,x_3 \in \{0,1\}^2} \mathbb{I}(x_2 \oplus x_3 = x_1) W(y_2|x_2) W(y_3|x_3) \tag{15}$$

$$= W(y_2|x_2 = x_1) \cdot W(y_3|x_3 = 0) + W(y_2|x_2 = x_1 \oplus 1) \cdot W(y_3|x_3 = 1) \tag{16}$$

$$\propto [W \boxast W](y_2, y_3|x_1), \tag{17}$$

where we need the factor 1/2 to make sure that it is an exact marginal (which we had omitted at the beginning of BP, in the MAP formulation, for convenience), or equivalently to ensure that $W \boxast W'$ is indeed a channel.

As discussed by Renes in [2], this perspective on BP extends to quantum observations and aids one in defining the channel combining operations for a classical-quantum (CQ) channel [3] $W(x) \equiv W(|x\rangle\langle x|), x \in \{0, 1\}$, as follows:

$$[W \circledast W'](x) := W(x) \otimes W'(x), \tag{18}$$

$$[W \circledast W'](x) \coloneqq \frac{1}{2} W(x) \otimes W'(0) + \frac{1}{2} W(x \oplus 1) \otimes W'(1). \tag{19}$$

Here, we have adopted the same notation as in [2], which suppresses the outputs "$(y, z)$" that were present in the classical channel convolutions (12) and (14). This is because we do not observe the output in the quantum case unless we measure it, and measuring each channel output is not always the optimal operation at the receiver.

**Remark 1.** Observe that, for a general CQ channel, $W(x)$ represents the output density matrix from the channel for the classical input $x \equiv |x\rangle\langle x|$. Thus, even if the channel outputs are pure states, the induced channel at the FNs still yields a mixed state. Also note that these channels are "automatically induced by the structure of the FG", and do not require any operation to be performed on the received states. Hence, the challenge is to identify the appropriate quantum "local inference" strategy, so that at the end of quantum BP we have performed appropriate statistical inference.

## Supplementary Note 3: Belief-Propagation with Quantum Messages (BPQM)

The idea of Renes [2] is to generalize the classical BP algorithm, which is exact for marginalization over tree FGs, to the quantum scenario. However, it is not clear how the posterior distribution should be defined in the quantum case because, unlike the classical case, we do not get "observations" unless we make measurements. We also know it is suboptimal to measure the output of each channel use and that collective measurements on all channel outputs may be required to achieve capacity [4]. The channel combining perspective provides a path forward. The primary difficulty is that the combined channels represent larger and larger systems after each operation. In the classical case, the output of a binary-input channel can always be replaced by a sufficient statistic that is a single real number. Thus, the BP messages for binary codes can be a single real number. In the general CQ case, that is not true. But, for pure-state channels, Renes showed that the combined channels can be compressed to output a single qubit along with a real number.

### Supplementary Note 3.1: Pure-State Classical-Quantum Channel

The pure-state channel is defined for classical inputs $x \equiv |x\rangle\langle x|, x \in \{0, 1\}$, as

$$\begin{aligned} W(x) &\coloneqq |\theta\rangle\langle 0| \cdot |x\rangle\langle x| \cdot |0\rangle\langle\theta| + |-\theta\rangle\langle 1| \cdot |x\rangle\langle x| \cdot |1\rangle\langle -\theta| && (20)\\ &= \langle x|0\rangle \cdot |\theta\rangle\langle\theta| + \langle x|1\rangle \cdot |-\theta\rangle\langle -\theta|, && (21)\\ |\pm\theta\rangle &\coloneqq \cos\frac{\theta}{2}|0\rangle \pm \sin\frac{\theta}{2}|1\rangle. && (22)\end{aligned}$$

Hence, the Kraus operators for the channel can be taken to be $M_0 = |\theta\rangle\langle 0|, M_1 = |-\theta\rangle\langle 1|$. If the input system to $W$ is denoted by $X$ and the output system by $B$, then the joint density matrix $\rho_{XB}$ that is required to characterize the entropic quantities for this channel is given by

$$\rho_{XB} \coloneqq q \cdot |0\rangle\langle 0|_X \otimes |\theta\rangle\langle\theta|_B + (1-q) \cdot |1\rangle\langle 1|_X \otimes |-\theta\rangle\langle -\theta|_B, \tag{23}$$

where $q$ is the prior probability for input $x = 0$. The joint (von Neumann) entropy for $XB$ is given by

$$\begin{aligned} S(XB)_\rho &= S(X) + \sum_{x\in\{0,1\}} p_X(x) S(\rho_B^{(x)}) && (24)\\ &= h_2(q) + q \cdot S(|\theta\rangle\langle\theta|_B) + (1-q) S(|-\theta\rangle\langle -\theta|_B) && (25)\\ &= h_2(q), && (26)\end{aligned}$$

where $h_2(q) \coloneqq -q\log_2(q) - (1-q)\log_2(1-q)$ (bits) is the binary entropy function and $S(|\theta\rangle\langle\theta|_B) = S(|-\theta\rangle\langle -\theta|_B) = 0$ since the states are pure. Therefore, the quantum mutual information for the pure-state channel is the symmetric Holevo information

$$\begin{aligned} I(X;B)_\rho &\coloneqq S(X)_\rho + S(B)_\rho - S(XB)_\rho && (27)\\ &= h_2(q) + S(\rho_B) - h_2(q) && (28)\\ &= S\left(q \cdot |\theta\rangle\langle\theta|_B + (1-q) \cdot |-\theta\rangle\langle -\theta|_B\right). && (29)\end{aligned}$$

The ultimate capacity for this channel in the asymptotic limit of a large number of channel uses (per use of the channel) is $\max_{q\in[0,1]} I(X;B)_\rho = \max_{q\in[0,1]} S(\rho_B)$. Since this channel is equivalent to the BPSK (binary phase shift keying) modulated pure-loss optical channel [5], it is known that the maximum occurs at $q = 1/2$ and hence the Holevo capacity is given by

$$C_\infty(W) = S\left(\frac{1}{2}\cdot|\theta\rangle\langle\theta|_B + \frac{1}{2}\cdot|-\theta\rangle\langle-\theta|_B\right) = h_2\left(\cos^2\frac{\theta}{2}\right) = h_2\left(\frac{1+\sqrt{F(W)}}{2}\right), \tag{30}$$

where the fidelity of the channel is $F(W) := |\langle\theta|-\theta\rangle|^2 = \cos^2\theta, \cos\theta = 2\cos^2\frac{\theta}{2} - 1$. The subscript "$\infty$" comes from defining $C_n$ to be the maximal normalized rate achievable by classical codes measuring groups of $n$ channel outputs collectively, and then observing that $C_n$ converges to the limit $C_\infty$ [6].

If, instead, we performed the Helstrom measurement at the output of each use of the channel, i.e., for each code bit sent through $W$, then this would induce a BSC($P_{\min}$) with $P_{\min} = (1-\sqrt{1-F(W)})/2$, which is the minimum probability of error to distinguish between the states $\{|\theta\rangle, |-\theta\rangle\}$. The Helstrom measurement [7, 8] to optimally distinguish between two density matrices $\rho_0$ and $\rho_1$ is defined by $\{\Pi_{\text{Hel}}, \mathbb{I}-\Pi_{\text{Hel}}\}$:

$$\Pi_{\text{Hel}} := \sum_{i:\,\lambda_i\geq 0} |i\rangle\langle i|\,, \quad (\rho_0-\rho_1)|i\rangle = \lambda_i|i\rangle\,. \tag{31}$$

For the pure state channel, it is easy to calculate that $\rho_0 - \rho_1 = |\theta\rangle\langle\theta| - |-\theta\rangle\langle-\theta| = \sin\theta\cdot X$ so that the Helstrom measurement is projecting onto the Pauli $X$ basis, i.e., the POVM is $\{|+\rangle\langle+|, |-\rangle\langle-|\}$. In practice, the Dolinar receiver for the BPSK modulated pure-loss optical channel induces this BSC($P_{\min}$) [5]. If we implemented a classical optimal (block-MAP) decoder on this induced BSC, then the capacity that is attainable is $C_1(W) = 1 - h_2(P_{\min})$, where the subscript "1" indicates that we are performing symbol-by-symbol measurements and not a collective measurement. It can be easily checked that $C_1(W) \ll C_\infty(W)$, and classical-quantum polar codes equipped with a quantum successive-cancellation decoder close this gap [4, 5]. However, the optimal decoder for CQ polar codes is hard to realize in the lab. Hence, an interesting open problem is to analyze how much of this gap is closed by BPQM because it can be mapped into a "successive-cancellation-type" decoder as discussed in [2]. In fact, we will see that BPQM has a successive-cancellation flavor by definition.

### Supplementary Note 3.2: Node Operations in BPQM

For the pure-state channel, the following operations are performed at variable nodes and factor nodes [2] (see Supplementary Note 6 for detailed calculations). At a VN, the convolution $W \circledast W'$ initially yields a CQ channel that only outputs either $|\theta\rangle\otimes|\theta'\rangle$ or $|-\theta\rangle\otimes|-\theta'\rangle$. Note that the local convolution is performed with respect to input $x = 0$ and $x = 1$ separately, respectively inducing signs $+$ and $-$. We say "initially" because we expect the signs of all incoming qubits at a VN to be the same, which means all independent local beliefs of the VN agree on the bit's value. Since the pure-state channel does not introduce noise, and the only uncertainty arises from the non-orthogonality of $|\theta\rangle$ and $|-\theta\rangle$, the qubits always combine in this ideal fashion until the first bit is decoded. But, whether this situation continues beyond the first bit depends upon whether the first bit was decoded to be a 0 or 1. This is because, as mentioned earlier, the FN channel convolution in (19) is defined assuming that the FN imposes an even parity-check. If, instead, it imposed an odd parity-check, as will happen when one of the bits is decoded to be a 1, then the FN convolution has to be modified appropriately. Therefore, if the FN originally had degree 3 and one of the bits was estimated to be 1, then we can remove the bit and update the FN to be an odd parity-check on two bits. This degree-2 FN effectively induces a modified VN convolution with the signs of the two qubits in disagreement.

Given the (ideal) convolution outputs, the following unitary is applied to "compress" the information into one qubit and force the other system to be in state $|0\rangle$:

$$U_\circledast(\theta,\theta') := \begin{bmatrix} a_+ & 0 & 0 & a_- \\ a_- & 0 & 0 & -a_+ \\ 0 & b_+ & b_- & 0 \\ 0 & b_- & -b_+ & 0 \end{bmatrix}, \tag{32}$$

$$a_\pm := \frac{1}{\sqrt{2}}\frac{\cos\left(\frac{\theta-\theta'}{2}\right) \pm \cos\left(\frac{\theta+\theta'}{2}\right)}{\sqrt{1+\cos\theta\cos\theta'}}, \quad b_\pm := \frac{1}{\sqrt{2}}\frac{\sin\left(\frac{\theta+\theta'}{2}\right) \mp \sin\left(\frac{\theta-\theta'}{2}\right)}{\sqrt{1-\cos\theta\cos\theta'}}. \tag{33}$$

Hence, we have $U_\circledast(\theta,\theta')\left(|\pm\theta\rangle\otimes|\pm\theta'\rangle\right) = |\pm\theta^\circledast\rangle\otimes|0\rangle$, where $\cos\theta^\circledast := \cos\theta\cos\theta'$. The VN update just passes the qubit in the first system and ignores the second system.

At the FN, the induced mixed state $[W \boxast W'](x)$ can be transformed into the CQ state $\sum_{j\in\{0,1\}} p_j \left|\pm\theta_j^{\boxast}\right\rangle \left\langle\pm\theta_j^{\boxast}\right| \otimes |j\rangle\langle j|$ by performing $U_{\boxast} := \mathrm{CNOT}_{W\to W'}$, the controlled-NOT gate with $W$ as control and $W'$ as target. Hence,

$$U_{\boxast}\left([W \boxast W'](x)\right) U_{\boxast}^{\dagger} = \sum_{j\in\{0,1\}} p_j \left|\pm\theta_j^{\boxast}\right\rangle \left\langle\pm\theta_j^{\boxast}\right| \otimes |j\rangle\langle j|, \tag{34}$$

$$p_0 := \frac{1}{2}(1+\cos\theta\cos\theta'),\ p_1 := 1-p_0, \quad \cos\theta_0^{\boxast} := \frac{\cos\theta+\cos\theta'}{1+\cos\theta\cos\theta'},\ \cos\theta_1^{\boxast} := \frac{\cos\theta-\cos\theta'}{1-\cos\theta\cos\theta'}. \tag{35}$$

Observe that for $j = 0$, the angle between the states has decreased, while for $j = 1$ the angle has increased. The FN update is then to measure the second system and pass the resulting qubit in the first system as the message, along with the result of the classical measurement (or the resulting value of $\theta^{\boxast}$). This is because the VN update at the next stage needs to know the angles $\theta, \theta'$ of the incoming qubits. When we have a degree $d$ node, these channel convolutions can be performed two at a time. Equivalently, we can write down a circuit composed of CNOT operations and $Z$-basis measurements, and use the "principle of deferred measurements" [9, Section 4.4] to delay the measurements until the end of the circuit. For clarity, we will describe BPQM as a coherent operation that does not measure or discard qubits along the way.

**Remark 2.** Note that in each half-iteration of BP, all VN or FN updates can be performed simultaneously since this involves only classical arithmetic and we can implicitly clone the values. This is indeed a different update schedule when compared to slower sequential updates, but can always be implemented if desired. However, in BPQM, we are forced to perform operations sequentially until one bit is decoded and then attempt to reverse the executed operations in a suitable manner. Our subsequent analysis of BPQM will assume this sequential schedule.

### Supplementary Note 4: The Intuitive Analysis for Bit 2 is Incorrect

Recollect that for $x_2$, we split $[W \boxast W](\hat{x}_1)_{23}$ in $\tilde{\rho}_{m_1,a}$ and arrived at the two hypotheses states

$$\tilde{\Phi}_{x_2=\hat{x}_1}(\hat{x}_1) = |m_1\theta\rangle\langle m_1\theta|_2 \otimes |\theta\rangle\langle\theta|_3 \otimes [W \boxast W](\hat{x}_1)_{45}, \tag{36}$$

$$\tilde{\Phi}_{x_2\neq\hat{x}_1}(\hat{x}_1) = |-m_1\theta\rangle\langle -m_1\theta|_2 \otimes |-\theta\rangle\langle-\theta|_3 \otimes [W \boxast W](\hat{x}_1)_{45}. \tag{37}$$

We can deterministically apply $Z^{\hat{x}_1}$ to system 2 in order to map this into the following state discrimination problem:

$$\Phi_{\pm}(\hat{x}_1) = |\pm\theta\rangle\langle\pm\theta|_2 \otimes |\pm\theta\rangle\langle\pm\theta|_3 \otimes [W \boxast W](\hat{x}_1)_{45}, \tag{38}$$

where $\pm \equiv (-1)^{x_2-\hat{x}_1}$. Clearly, we can process systems 2 and 3 alone to decide $x_2$, and similarly systems 4 and 5 alone to decide $x_4$. It is also clear that by performing the variable node operation $U_{\circledast}(\theta,\theta)$, we compress all the information into system 2, i.e., produce $|\pm\theta^{\circledast}\rangle\langle\pm\theta^{\circledast}|_2 \otimes |0\rangle\langle 0|_3$, which can then be optimally distinguished by measuring in the $X$-basis. (Note that we are using the same notation $\theta^{\circledast}$ as in Supplementary Note 3.2 but here $\theta' = \theta$.) This agrees with the definition of node operations in BPQM as well because now the factor node $\tilde{c}_1$ in Fig. 7 (of the main text) has degree 2, and hence the optimal processing is to perform the variable node convolution between qubits 2 and 3. We can incorporate the operation $Z^{\hat{x}_1}$ into BPQM by performing $U_{\circledast}(m_1\theta,\theta)$ on systems 2 and 3 (and similarly on systems 4 and 5). Although $U_{\circledast}(m_1\theta,\theta) \neq U_{\circledast}(\theta,\theta)\cdot(Z^{\hat{x}_1}\otimes I_2)$, the two operations act identically on the states $\tilde{\Phi}_{x_2=\hat{x}_1}(\hat{x}_1)$ and $\tilde{\Phi}_{x_2\neq\hat{x}_1}(\hat{x}_1)$.

Hence, since the operation in Supplementary Figure 3 is optimal (Helstrom) for distinguishing $\tilde{\Phi}_{x_2=\hat{x}_1}(\hat{x}_1)$ and $\tilde{\Phi}_{x_2\neq\hat{x}_1}(\hat{x}_1)$, we expect the BPQM success probability for decoding $\hat{x}_2 = x_2$ to be

$$\mathbb{P}[\hat{x}_2 = x_2] = \frac{1}{2} + \frac{1}{4}\left\|\tilde{\Phi}_{x_2=\hat{x}_1}(\hat{x}_1) - \tilde{\Phi}_{x_2\neq\hat{x}_1}(\hat{x}_1)\right\|_1 \tag{39}$$

$$= \frac{1}{2} + \frac{1}{4}\left\|\Phi_{+}(\hat{x}_1) - \Phi_{-}(\hat{x}_1)\right\|_1 \tag{40}$$

$$= \frac{1}{2} + \frac{1}{4}\left\|(|\theta^{\circledast}\rangle\langle\theta^{\circledast}| - |-\theta^{\circledast}\rangle\langle-\theta^{\circledast}|)_2 \otimes |0\rangle\langle 0|_3 \otimes [W \boxast W](\hat{x}_1)_{45}\right\|_1 \tag{41}$$

$$= \frac{1}{2} + \frac{1}{4}\cdot\sin\theta^{\circledast}\,\|X\|_1 \tag{42}$$

$$= \frac{1+\sin\theta^{\circledast}}{2} = \frac{1+\sqrt{1-\cos^4\theta}}{2}. \tag{43}$$

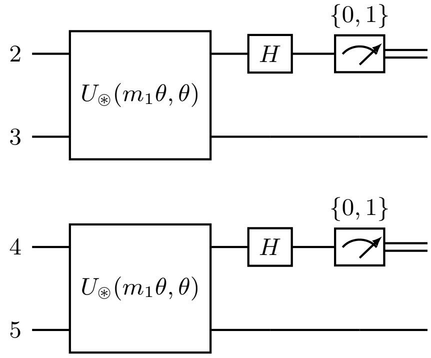


Supplementary Figure 3: The circuit performed in BPQM after decoding bit $x_1$ and reversing the operations performed prior to measurement.

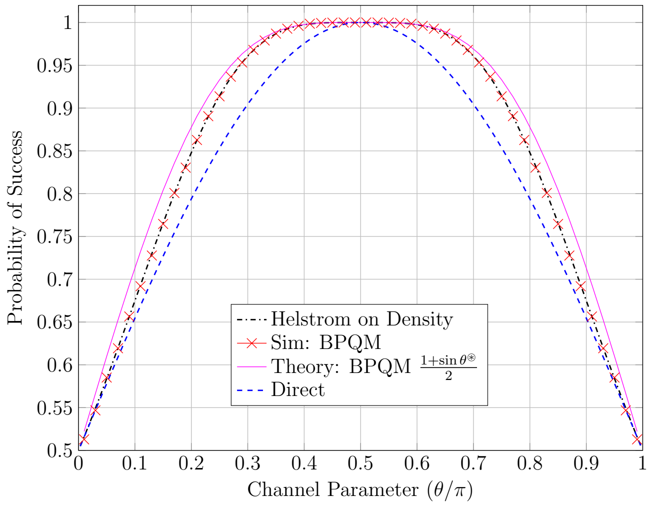


(a) The success probabilities for decoding the value of $x_2$ or $x_4$.

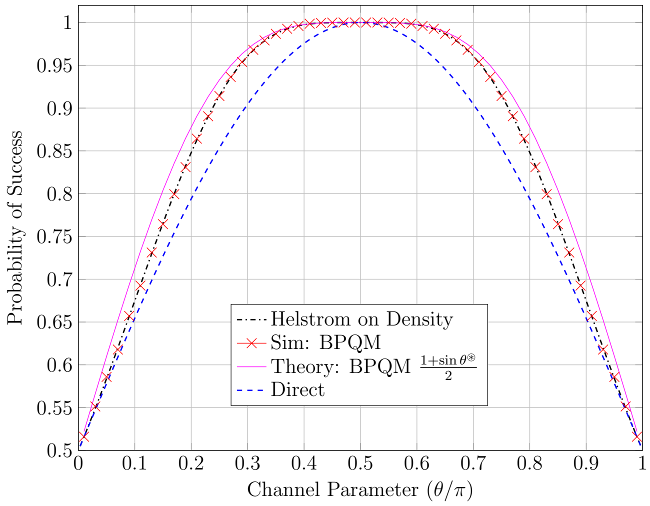


(b) The success probabilities for decoding the value of $x_3$ or $x_5$.

Supplementary Figure 4: The success probabilities for decoding the value of $x_2$ or $x_4$ (a) and $x_3$ or $x_5$ (b) in the 5-bit code. Here, "Helstrom on Density" represents $P^{\text{Hel}}_{\text{succ},k}$ and "Direct" represents the success probability when directly implementing the Helstrom measurement at the channel output on system $k$, for $k \in \{2, 3, 4, 5\}$. The curves "Sim: BPQM" correspond to a simulation that averaged each data point over $10^5$ uniformly random codeword transmissions.

Note that if we had defined the state $\tilde{\rho}_{m_1,a}$ to be conditioned on the cases $\hat{x}_1 = x_1$ and $\hat{x}_1 \neq x_1$ separately, then using a similar calculation as above we would still obtain

$$\mathbb{P}[\hat{x}_2 = x_2] = \mathbb{P}[\hat{x}_1 = x_1] \cdot \mathbb{P}[\hat{x}_2 = x_2 \,|\, \hat{x}_1 = x_1] + \mathbb{P}[\hat{x}_1 \neq x_1] \cdot \mathbb{P}[\hat{x}_2 = x_2 \,|\, \hat{x}_1 \neq x_1] \tag{44}$$

$$= P^{\text{BPQM}}_{\text{succ},1} \cdot \frac{1}{2}\left(1 + \frac{\sin\theta^{\circledast}}{P^{\text{BPQM}}_{\text{succ},1}}\right) + \left(1 - P^{\text{BPQM}}_{\text{succ},1}\right) \cdot \frac{1}{2} = \frac{1 + \sin\theta^{\circledast}}{2}. \tag{45}$$

Finally, bits $x_3$ and $x_5$ can be estimated simply as $\hat{x}_3 = \hat{x}_2 \oplus \hat{x}_1$ and $\hat{x}_5 = \hat{x}_4 \oplus \hat{x}_1$, without performing any quantum operations. Due to symmetry, the success probabilities for both these bits are the same. Bit 3 is decoded correctly, i.e., $\hat{x}_3 = x_3$, if either $\hat{x}_1 = x_1$ and $\hat{x}_2 = x_2$ or $\hat{x}_1 \neq x_1$ and $\hat{x}_2 \neq x_2$. Hence, we can write

$$\mathbb{P}[\hat{x}_3 = x_3] = \mathbb{P}[\hat{x}_1 = x_1] \cdot \mathbb{P}[\hat{x}_2 = x_2 \,|\, \hat{x}_1 = x_1] + \mathbb{P}[\hat{x}_1 \neq x_1] \cdot \mathbb{P}[\hat{x}_2 \neq x_2 \,|\, \hat{x}_1 \neq x_1] \tag{46}$$

$$= P^{\text{BPQM}}_{\text{succ},1} \cdot \frac{1}{2}\left(1 + \frac{\sin\theta^{\circledast}}{P^{\text{BPQM}}_{\text{succ},1}}\right) + \left(1 - P^{\text{BPQM}}_{\text{succ},1}\right) \cdot \frac{1}{2} \tag{47}$$

$$= \frac{1+\sin\theta^{\circledast}}{2}. \tag{48}$$

Again, $P^{\text{Hel}}_{\text{succ},5} = P^{\text{Hel}}_{\text{succ},3}$, and these probabilites are plotted in Supplementary Figure 4 (right).

We simulated the performance of BPQM by randomly generating $10^5$ codewords, passing each of them through 5 independent copies of the pure state channel, and employing the above sequence of unitaries and measurements for decoding all the bits. We plot the empirical performance of BPQM for decoding bit 2 in Supplementary Figure 4 (left), along with the predicted theoretical performance above, the performance for directly measuring the second qubit at the channel output, and also the Helstrom success probability $P^{\text{Hel}}_{\text{succ},2}$ for optimally distinguishing $\rho_2^{(0)}$ and $\rho_2^{(1)}$, where

$$\rho_2^{(0)} = |\theta\rangle\langle\theta|_2 \otimes \left[\frac{1}{2}|\theta\rangle\langle\theta|_1 \otimes |\theta\rangle\langle\theta|_3 \otimes [W \circledast W](0)_{45} + \frac{1}{2}|-\theta\rangle\langle-\theta|_1 \otimes |-\theta\rangle\langle-\theta|_3 \otimes [W \circledast W](1)_{45}\right], \tag{49}$$

$$\rho_2^{(1)} = |-\theta\rangle\langle-\theta|_2 \otimes \left[\frac{1}{2}|\theta\rangle\langle\theta|_1 \otimes |-\theta\rangle\langle-\theta|_3 \otimes [W \circledast W](0)_{45} + \frac{1}{2}|-\theta\rangle\langle-\theta|_1 \otimes |\theta\rangle\langle\theta|_3 \otimes [W \circledast W](1)_{45}\right]. \tag{50}$$

We observe that BPQM performs significantly better than direct Helstrom measurement of the channel output, as we might expect. Moreover, the performance of BPQM is indistinguishable (up to numerical precision) from that of the Helstrom measurement that optimally distinguishes between $\rho_2^{(0)}$ and $\rho_2^{(1)}$. This suggests that BPQM might be provably optimal for decoding bit 2 as well, even though the measurement for bit 1 rendered the original channel outputs irrecoverable. However, we also notice that the above prediction for the BPQM success probability for decoding bit 2 is relatively higher than even the optimal Helstrom measurement. This indicates that the state discrimination problem for bit 2 discussed above is more ideal than the actual problem in hand. Hence, we analyze the true state discrimination problem for bit 2 (or 4) in Section III-C (of the main text) and clarify the observed performance in Supplementary Figure 4.

### Supplementary Note 5: Circuit Decomposition for Variable Node Unitary and Conditional Rotation

Let $\text{CNOT}_{\theta' \to \theta} = I_2 \otimes |0\rangle\langle 0| + X \otimes |1\rangle\langle 1|$ be the controlled-NOT operation with the (second) qubit corresponding to angle $\theta'$ as the control qubit. Then we observe that

$$\tilde{U}_{\circledast}(\theta,\theta') := U_{\circledast}(\theta,\theta')\,\text{CNOT}_{\theta'\to\theta} = \begin{bmatrix} a_+ & a_- & 0 & 0 \\ a_- & -a_+ & 0 & 0 \\ 0 & 0 & b_- & b_+ \\ 0 & 0 & -b_+ & b_- \end{bmatrix}, \tag{51}$$

$$= |0\rangle\langle 0| \otimes \begin{bmatrix} a_+ & a_- \\ a_- & -a_+ \end{bmatrix} + |1\rangle\langle 1| \otimes \begin{bmatrix} b_- & b_+ \\ -b_+ & b_- \end{bmatrix} \tag{52}$$

$$=: |0\rangle\langle 0| \otimes U_1 + |1\rangle\langle 1| \otimes U_2 \tag{53}$$

$$= (|0\rangle\langle 0| \otimes U_1 + |1\rangle\langle 1| \otimes I_2)\,(|0\rangle\langle 0| \otimes I_2 + |1\rangle\langle 1| \otimes U_2)\,. \tag{54}$$

Let $R_p(\theta) := \exp\left(-\imath\frac{\theta}{2}p\right)$ denote Pauli rotations, where $p \in \{x,y,z\}$ and $\imath := \sqrt{-1}$. Then the $Z$-$Y$ decomposition for a single qubit [9, Theorem 4.1] implies that any unitary $U$ can be decomposed as

$$U = e^{\imath\alpha} R_z(\beta) R_y(\gamma) R_z(\delta) = \begin{bmatrix} e^{\imath(\alpha-\beta/2-\delta/2)}\cos\frac{\gamma}{2} & -e^{\imath(\alpha-\beta/2+\delta/2)}\sin\frac{\gamma}{2} \\ e^{\imath(\alpha+\beta/2-\delta/2)}\sin\frac{\gamma}{2} & e^{\imath(\alpha+\beta/2+\delta/2)}\cos\frac{\gamma}{2} \end{bmatrix}. \tag{55}$$

Setting $\gamma_1 := 2\sin^{-1}(a_-)$ and $\gamma_2 := 2\sin^{-1}(b_+)$, we observe that [9, Corollary 4.2]

$$U_1 = \begin{bmatrix} \cos\frac{\gamma_1}{2} & \sin\frac{\gamma_1}{2} \\ \sin\frac{\gamma_1}{2} & -\cos\frac{\gamma_1}{2} \end{bmatrix} = e^{\frac{\imath\pi}{2}} R_y(\gamma_1) R_z(\pi) =: e^{\frac{\imath\pi}{2}} A_1 X B_1 X C_1, \tag{56}$$

$$A_1 := R_y\left(\frac{\gamma_1}{2}\right), \tag{57}$$

$$B_1 := R_y\left(\frac{-\gamma_1}{2}\right) R_z\left(\frac{-\pi}{2}\right), \tag{58}$$

$$C_1 := R_z\left(\frac{\pi}{2}\right), \tag{59}$$

$$U_2 = \begin{bmatrix} \cos\frac{\gamma_2}{2} & \sin\frac{\gamma_2}{2} \\ -\sin\frac{\gamma_2}{2} & \cos\frac{\gamma_2}{2} \end{bmatrix} = e^{\imath\pi} R_z(\pi) R_y(\gamma_2) R_z(\pi) =: e^{\imath\pi} A_2 X B_2 X, \tag{60}$$

$$A_2 \coloneqq R_z(\pi) R_y(\gamma_2/2), \tag{61}$$

$$B_2 \coloneqq R_y(-\gamma_2/2) R_z(-\pi). \tag{62}$$

Then we can express the full circuit decomposition for $U_{\circledast}(\theta, \theta')$ as shown in Fig. 9 (of the main text).

Similarly, the rotations $K_+$ and $K_-$ defined in eqn. (21) can be expressed as

$$K_+ = \frac{1}{\sqrt{2}} \begin{bmatrix} \cos\frac{\varphi_{00}^{\circledast}}{2} + \sin\frac{\varphi_{00}^{\circledast}}{2} & \cos\frac{\varphi_{00}^{\circledast}}{2} - \sin\frac{\varphi_{00}^{\circledast}}{2} \\ \sin\frac{\varphi_{00}^{\circledast}}{2} - \cos\frac{\varphi_{00}^{\circledast}}{2} & \sin\frac{\varphi_{00}^{\circledast}}{2} + \cos\frac{\varphi_{00}^{\circledast}}{2} \end{bmatrix} \tag{63}$$

$$=: \begin{bmatrix} \cos\frac{\gamma}{2} & \sin\frac{\gamma}{2} \\ -\sin\frac{\gamma}{2} & \cos\frac{\gamma}{2} \end{bmatrix} \tag{64}$$

$$= e^{\imath\pi} R_z(\pi) R_y(\gamma) R_z(\pi) \tag{65}$$

$$=: e^{\imath\pi} A_+ X B_+ X, \tag{66}$$

$$K_- = \frac{1}{\sqrt{2}} \begin{bmatrix} \sin\frac{\varphi_{00}^{\circledast}}{2} + \cos\frac{\varphi_{00}^{\circledast}}{2} & \sin\frac{\varphi_{00}^{\circledast}}{2} - \cos\frac{\varphi_{00}^{\circledast}}{2} \\ \cos\frac{\varphi_{00}^{\circledast}}{2} - \sin\frac{\varphi_{00}^{\circledast}}{2} & \cos\frac{\varphi_{00}^{\circledast}}{2} + \sin\frac{\varphi_{00}^{\circledast}}{2} \end{bmatrix} \tag{67}$$

$$= K_+^\dagger, \tag{68}$$

$$\text{where} \;\; \gamma \coloneqq 2\sin^{-1}\left[\frac{1}{\sqrt{2}}\left(\cos\frac{\varphi_{00}^{\circledast}}{2} - \sin\frac{\varphi_{00}^{\circledast}}{2}\right)\right], \tag{69}$$

$$A_+ \coloneqq R_z(\pi) R_y\left(\frac{\gamma}{2}\right), \tag{70}$$

$$B_+ \coloneqq R_y\left(\frac{-\gamma}{2}\right) R_z(-\pi). \tag{71}$$

The coherently controlled gate $M_{m_1}$ defined in eqn. (21) is decomposed in Fig. 10 (of the main text) using the above calculations.

## Supplementary Note 6: Calculations for Node Convolutions

The variable and check node convolutions are given by

$$[W \circledast W'](x) = W(x) \otimes W'(x), \tag{72}$$

$$[W \boxast W'](x) = \frac{1}{2}(W(x) \otimes W'(0) + W(x+1) \otimes W'(1)). \tag{73}$$

The channel outputs for a pure state channel are $|\pm\theta\rangle$, where

$$|\pm\theta\rangle = \cos\frac{\theta}{2}|0\rangle \pm \sin\frac{\theta}{2}|1\rangle. \tag{74}$$

The overlap between the two outputs is given by $\langle -\theta|\theta\rangle = \cos^2\frac{\theta}{2} - \sin^2\frac{\theta}{2} = \cos\theta$. The Helstrom measurement projects onto $\left|\pm\frac{\pi}{2}\right\rangle$.

The Stinespring's representation for a classical-quantum (CQ) channel $W$ that maps density states from Hilbert space $\mathcal{H}_A$ to $\mathcal{H}_B$ is given by

$$W(x) \coloneqq \mathrm{Tr}_E\left[V_{BE|A}|x\rangle\langle x| V_{BE|A}^\dagger\right], \tag{75}$$

where $\mathcal{H}_E$ is an ancilla space and $V_{BE|A}$ is an isometry that maps $\mathcal{H}_A$ to $\mathcal{H}_B \otimes \mathcal{H}_E$. Therefore, even for a pure state channel $W$, we must take its outputs to be density states $|\pm\theta\rangle\langle\pm\theta|$ and not $|\pm\theta\rangle$. On the contrary, if we take it to be $|\pm\theta\rangle$ then we immediately notice that the output state of the check convolution in (73) above is not normalized and hence does not represent a physical operation.

*Variable Node Convolution:* The convolution $W \circledast W'$ outputs (the density state for) either $|\theta^{\circledast}\rangle := |\theta\rangle \otimes |\theta'\rangle$ or $|{-\theta^{\circledast}}\rangle := |{-\theta}\rangle \otimes |{-\theta'}\rangle$, which are again two pure states with an overlap angle $\theta^{\circledast}$ given by

$$\cos\theta^{\circledast} := \langle -\theta^{\circledast}|\theta^{\circledast}\rangle = (\langle -\theta| \otimes \langle -\theta'|) \cdot (|\theta\rangle \otimes |\theta'\rangle) = \langle -\theta|\theta\rangle \otimes \langle -\theta'|\theta'\rangle = \cos\theta\cos\theta'. \tag{76}$$

The following unitary transformation compresses the states to the first qubit, leaving the second in the state $|0\rangle$:

$$U_{\circledast}(\theta,\theta') := \begin{bmatrix} a_+ & 0 & 0 & a_- \\ a_- & 0 & 0 & -a_+ \\ 0 & b_+ & b_- & 0 \\ 0 & b_- & -b_+ & 0 \end{bmatrix}, \tag{77}$$

where

$$a_{\pm} = \frac{1}{\sqrt{2}} \frac{\cos\left(\frac{\theta-\theta'}{2}\right) \pm \cos\left(\frac{\theta+\theta'}{2}\right)}{\sqrt{1+\cos\theta\cos\theta'}}, \quad b_{\pm} = \frac{1}{\sqrt{2}} \frac{\sin\left(\frac{\theta+\theta'}{2}\right) \mp \sin\left(\frac{\theta-\theta'}{2}\right)}{\sqrt{1-\cos\theta\cos\theta'}}. \tag{78}$$

Let us verify by explicit calculation that

$$U_{\circledast}(\theta,\theta') \left(|\pm\theta\rangle\langle\pm\theta| \otimes |\pm\theta'\rangle\langle\pm\theta'|\right) U_{\circledast}^{\dagger}(\theta,\theta') = \left|\pm\theta^{\circledast}\right\rangle\left\langle\pm\theta^{\circledast}\right| \otimes |0\rangle\langle 0|, \tag{79}$$

where $|\pm\theta^{\circledast}\rangle := \sqrt{p_0}\,|0\rangle \pm \sqrt{p_1}\,|1\rangle$, $p_0 := \frac{1}{2}(1+\cos\theta\cos\theta')$, $p_1 := 1-p_0 = \frac{1}{2}(1-\cos\theta\cos\theta')$.

$$\left|\pm\theta^{\circledast}\right\rangle := \begin{bmatrix} \sqrt{\frac{1+\cos\theta\cos\theta'}{2}} \\ \pm\sqrt{\frac{1-\cos\theta\cos\theta'}{2}} \end{bmatrix} = \begin{bmatrix} \sqrt{\frac{1+\cos\theta^{\circledast}}{2}} \\ \pm\sqrt{\frac{1-\cos\theta^{\circledast}}{2}} \end{bmatrix} = \begin{bmatrix} \cos\frac{\theta^{\circledast}}{2} \\ \pm\sin\frac{\theta^{\circledast}}{2} \end{bmatrix} = \cos\frac{\theta^{\circledast}}{2}|0\rangle \pm \sin\frac{\theta^{\circledast}}{2}|1\rangle. \tag{80}$$

First, using the definitions for $|\pm\theta\rangle$ and $|\pm\theta'\rangle$ we have

$$\begin{aligned} |\pm\theta\rangle \otimes |\pm\theta'\rangle &= \cos\frac{\theta}{2}\cos\frac{\theta'}{2}|00\rangle \pm \cos\frac{\theta}{2}\sin\frac{\theta'}{2}|01\rangle \pm \sin\frac{\theta}{2}\cos\frac{\theta'}{2}|10\rangle + \sin\frac{\theta}{2}\sin\frac{\theta'}{2}|11\rangle & (81)\\ &= \left[\cos\frac{\theta}{2}\cos\frac{\theta'}{2},\ \pm\cos\frac{\theta}{2}\sin\frac{\theta'}{2},\ \pm\sin\frac{\theta}{2}\cos\frac{\theta'}{2},\ \sin\frac{\theta}{2}\sin\frac{\theta'}{2}\right]^T. & (82) \end{aligned}$$

Hence we get

$$|\pm\psi\rangle := U_{\circledast}(\theta,\theta')\left(|\pm\theta\rangle \otimes |\pm\theta'\rangle\right) = \begin{bmatrix} a_+\cos\frac{\theta}{2}\cos\frac{\theta'}{2} + a_-\sin\frac{\theta}{2}\sin\frac{\theta'}{2} \\ a_-\cos\frac{\theta}{2}\cos\frac{\theta'}{2} - a_+\sin\frac{\theta}{2}\sin\frac{\theta'}{2} \\ \pm b_+\cos\frac{\theta}{2}\sin\frac{\theta'}{2} \pm b_-\sin\frac{\theta}{2}\cos\frac{\theta'}{2} \\ \pm b_-\cos\frac{\theta}{2}\sin\frac{\theta'}{2} \mp b_+\sin\frac{\theta}{2}\cos\frac{\theta'}{2} \end{bmatrix} =: \begin{bmatrix} \psi_{00} \\ \psi_{01} \\ \psi_{10} \\ \psi_{11} \end{bmatrix}. \tag{83}$$

For convenience let us make some definitions:

$$\begin{aligned} \alpha &:= \cos\frac{\theta-\theta'}{2} + \cos\frac{\theta+\theta'}{2} = \frac{1}{2}\cos\frac{\theta}{2}\cos\frac{\theta'}{2}, \quad \beta := \cos\frac{\theta-\theta'}{2} - \cos\frac{\theta+\theta'}{2} = \frac{1}{2}\sin\frac{\theta}{2}\sin\frac{\theta'}{2}, & (84)\\ \gamma &:= \sin\frac{\theta+\theta'}{2} - \sin\frac{\theta-\theta'}{2} = \frac{1}{2}\cos\frac{\theta}{2}\sin\frac{\theta'}{2}, \quad \delta := \sin\frac{\theta+\theta'}{2} + \sin\frac{\theta-\theta'}{2} = \frac{1}{2}\sin\frac{\theta}{2}\cos\frac{\theta'}{2}. & (85) \end{aligned}$$

Then using the identities $\cos\theta = 2\cos^2\frac{\theta}{2} - 1 = 1 - 2\sin^2\frac{\theta}{2}$ we see that

$$\begin{aligned} \psi_{00} &= \frac{1}{2}\left[a_+\alpha + a_-\beta\right] = \frac{1}{2\sqrt{2}} \frac{2\left[\cos^2\frac{\theta-\theta'}{2} + \cos^2\frac{\theta+\theta'}{2}\right]}{\sqrt{1+\cos\theta\cos\theta'}} = \sqrt{\frac{1+\cos\theta\cos\theta'}{2}}, & (86)\\ \psi_{01} &= \frac{1}{2}\left[a_-\alpha - a_+\beta\right] = \frac{1}{2\sqrt{2}} \frac{\alpha\beta - \beta\alpha}{\sqrt{1+\cos\theta\cos\theta'}} = 0, & (87)\\ \psi_{10} &= \frac{1}{2}\left[\pm b_+\gamma \pm b_-\delta\right] = \frac{1}{2\sqrt{2}} \frac{2\left[\pm\sin^2\frac{\theta+\theta'}{2} \pm \sin^2\frac{\theta-\theta'}{2}\right]}{\sqrt{1-\cos\theta\cos\theta'}} = \pm\sqrt{\frac{1-\cos\theta\cos\theta'}{2}}, & (88)\\ \psi_{11} &= \frac{1}{2}\left[\pm b_-\gamma \mp b_+\delta\right] = \frac{1}{2\sqrt{2}} \frac{\pm\gamma\delta \mp \delta\gamma}{\sqrt{1-\cos\theta\cos\theta'}} = 0. & (89) \end{aligned}$$

Therefore we find that $|\pm\psi\rangle = |\pm\theta^{\circledast}\rangle \otimes |0\rangle$ and hence

$$U_{\circledast}(\theta,\theta')\left(|\pm\theta\rangle\langle\pm\theta| \otimes |\pm\theta'\rangle\langle\pm\theta'|\right)U_{\circledast}^{\dagger}(\theta,\theta') = |\pm\psi\rangle\langle\pm\psi| = \left|\pm\theta^{\circledast}\right\rangle\left\langle\pm\theta^{\circledast}\right| \otimes |0\rangle\langle 0|. \tag{90}$$

*Factor Node Convolution:* The result of $W \circledast W$ is not pure and hence we would like to unitarily transform the output of the $\circledast$ convolution to a CQ state of the form

$$\Psi_{\text{desired}} := \sum_{j\in\{0,1\}} p_j \left|\pm\theta_j^{\circledast}\right\rangle \left\langle\pm\theta_j^{\circledast}\right| \otimes |j\rangle\langle j|, \tag{91}$$

for some appropriate state $\left|\pm\theta_j^{\circledast}\right\rangle$ and probabilities $p_j$. It turns out that the unitary operation $U_{\circledast} := \text{CNOT}_{1\to 2}$ is the correct one. Let us verify that by explicit calculation for inputs $x = 0$ and $x = 1$ simultaneously. We have

$$[W \circledast W'](x) = \frac{1}{2}\left(W(x)\otimes W'(0) + W(x\oplus 1)\otimes W'(1)\right) \tag{92}$$

$$= \frac{1}{2}\bigg( |\pm\theta\rangle\langle\pm\theta| \otimes |\theta'\rangle\langle\theta'| + |\mp\theta\rangle\langle\mp\theta|\otimes|-\theta'\rangle\langle-\theta'|\bigg) \quad (\pm \equiv (-1)^x,\ \mp\equiv(-1)^{x\oplus 1}) \tag{93}$$

$$:= \frac{1}{2}\left(\tilde{\varphi}_1 + \tilde{\varphi}_2\right). \tag{94}$$

$$\Rightarrow \Psi := U_{\circledast}\bigg([W\circledast W'](x)\bigg)U_{\circledast}^{\dagger} \tag{95}$$

$$= \frac{1}{2}\left(U_{\circledast}\tilde{\varphi}_1 U_{\circledast}^{\dagger} + U_{\circledast}\tilde{\varphi}_2 U_{\circledast}^{\dagger}\right) \tag{96}$$

$$:= \frac{1}{2}\left(\varphi_1 + \varphi_2\right). \tag{97}$$

Now we calculate $\varphi_1$ and $\varphi_2$ separately. We first have

$$\begin{aligned}
\tilde{\varphi}_1 &= |\pm\theta\rangle\langle\pm\theta|\otimes|\theta'\rangle\langle\theta'| \\
&= (|\pm\theta\rangle\otimes|\theta'\rangle)\cdot(\langle\pm\theta|\otimes\langle\theta'|) &(98)\\
&= \left[\cos\frac{\theta}{2}\cos\frac{\theta'}{2}|0\rangle|0\rangle + \cos\frac{\theta}{2}\sin\frac{\theta'}{2}|0\rangle|1\rangle \pm \sin\frac{\theta}{2}\cos\frac{\theta'}{2}|1\rangle|0\rangle \pm \sin\frac{\theta}{2}\sin\frac{\theta'}{2}|1\rangle|1\rangle\right] \\
&\quad\otimes\left[\cos\frac{\theta}{2}\cos\frac{\theta'}{2}\langle 0|\langle 0| + \cos\frac{\theta}{2}\sin\frac{\theta'}{2}\langle 0|\langle 1| \pm \sin\frac{\theta}{2}\cos\frac{\theta'}{2}\langle 1|\langle 0| \pm \sin\frac{\theta}{2}\sin\frac{\theta'}{2}\langle 1|\langle 1|\right] &(99)\\
\Rightarrow \varphi_1 &= \text{CNOT}_{1\to 2}\left(\tilde{\varphi}_1\right)\text{CNOT}_{1\to 2} \\
&= \left[\cos\frac{\theta}{2}\cos\frac{\theta'}{2}|0\rangle|0\rangle + \cos\frac{\theta}{2}\sin\frac{\theta'}{2}|0\rangle|1\rangle \pm \sin\frac{\theta}{2}\sin\frac{\theta'}{2}|1\rangle|0\rangle \pm \sin\frac{\theta}{2}\cos\frac{\theta'}{2}|1\rangle|1\rangle\right] \\
&\quad\otimes\left[\cos\frac{\theta}{2}\cos\frac{\theta'}{2}\langle 0|\langle 0| + \cos\frac{\theta}{2}\sin\frac{\theta'}{2}\langle 0|\langle 1| \pm \sin\frac{\theta}{2}\sin\frac{\theta'}{2}\langle 1|\langle 0| \pm \sin\frac{\theta}{2}\cos\frac{\theta'}{2}\langle 1|\langle 1|\right] &(100)\\
&= \left[\cos^2\frac{\theta}{2}\cos^2\frac{\theta'}{2}|0\rangle\langle 0| \pm \frac{1}{4}\sin\theta\sin\theta'(|0\rangle\langle 1| + |1\rangle\langle 0|) + \sin^2\frac{\theta}{2}\sin^2\frac{\theta'}{2}|1\rangle\langle 1|\right]\otimes|0\rangle\langle 0| \\
&+ \left[\cos^2\frac{\theta}{2}\sin^2\frac{\theta'}{2}|0\rangle\langle 0| \pm \frac{1}{4}\sin\theta\sin\theta'(|0\rangle\langle 1| + |1\rangle\langle 0|) + \sin^2\frac{\theta}{2}\cos^2\frac{\theta'}{2}|1\rangle\langle 1|\right]\otimes|1\rangle\langle 1| \\
&+ \frac{1}{2}\left[\cos^2\frac{\theta}{2}\sin\theta'|0\rangle\langle 0| \pm \sin\theta\cos^2\frac{\theta'}{2}|0\rangle\langle 1| \pm \sin\theta\sin^2\frac{\theta'}{2}|1\rangle\langle 0| + \sin^2\frac{\theta}{2}\sin\theta'|1\rangle\langle 1|\right]\otimes|0\rangle\langle 1| \\
&+ \frac{1}{2}\left[\cos^2\frac{\theta}{2}\sin\theta'|0\rangle\langle 0| \pm \sin\theta\sin^2\frac{\theta'}{2}|0\rangle\langle 1| \pm \sin\theta\cos^2\frac{\theta'}{2}|1\rangle\langle 0| + \sin^2\frac{\theta}{2}\sin\theta'|1\rangle\langle 1|\right]\otimes|1\rangle\langle 0|. &(101)
\end{aligned}$$

Similarly we get

$$\begin{aligned}
\tilde{\varphi}_2 &= |\mp\theta\rangle\langle\mp\theta|\otimes|-\theta'\rangle\langle-\theta'| \\
&= (|\mp\theta\rangle\otimes|-\theta'\rangle)\cdot(\langle\mp\theta|\otimes\langle-\theta'|) &(102)\\
&= \left[\cos\frac{\theta}{2}\cos\frac{\theta'}{2}|0\rangle|0\rangle - \cos\frac{\theta}{2}\sin\frac{\theta'}{2}|0\rangle|1\rangle \mp \sin\frac{\theta}{2}\cos\frac{\theta'}{2}|1\rangle|0\rangle \pm \sin\frac{\theta}{2}\sin\frac{\theta'}{2}|1\rangle|1\rangle\right] \\
&\quad\otimes\left[\cos\frac{\theta}{2}\cos\frac{\theta'}{2}\langle 0|\langle 0| - \cos\frac{\theta}{2}\sin\frac{\theta'}{2}\langle 0|\langle 1| \mp \sin\frac{\theta}{2}\cos\frac{\theta'}{2}\langle 1|\langle 0| \pm \sin\frac{\theta}{2}\sin\frac{\theta'}{2}\langle 1|\langle 1|\right] &(103)\\
\Rightarrow \varphi_2 &= \text{CNOT}_{1\to 2}\left(\tilde{\varphi}_2\right)\text{CNOT}_{1\to 2}
\end{aligned}$$

$$
\begin{aligned}
&= \left[\cos\frac{\theta}{2}\cos\frac{\theta'}{2}\left|0\right\rangle\left|0\right\rangle - \cos\frac{\theta}{2}\sin\frac{\theta'}{2}\left|0\right\rangle\left|1\right\rangle \pm \sin\frac{\theta}{2}\sin\frac{\theta'}{2}\left|1\right\rangle\left|0\right\rangle \mp \sin\frac{\theta}{2}\cos\frac{\theta'}{2}\left|1\right\rangle\left|1\right\rangle\right] \\
&\quad\otimes \left[\cos\frac{\theta}{2}\cos\frac{\theta'}{2}\left\langle 0\right|\left\langle 0\right| - \cos\frac{\theta}{2}\sin\frac{\theta'}{2}\left\langle 0\right|\left\langle 1\right| \pm \sin\frac{\theta}{2}\sin\frac{\theta'}{2}\left\langle 1\right|\left\langle 0\right| \mp \sin\frac{\theta}{2}\cos\frac{\theta'}{2}\left\langle 1\right|\left\langle 1\right|\right] \qquad (104) \\
&= \left[\cos^2\frac{\theta}{2}\cos^2\frac{\theta'}{2}\left|0\right\rangle\left\langle 0\right| \pm \frac{1}{4}\sin\theta\sin\theta'(\left|0\right\rangle\left\langle 1\right| + \left|1\right\rangle\left\langle 0\right|) + \sin^2\frac{\theta}{2}\sin^2\frac{\theta'}{2}\left|1\right\rangle\left\langle 1\right|\right] \otimes \left|0\right\rangle\left\langle 0\right| \\
&+ \left[\cos^2\frac{\theta}{2}\sin^2\frac{\theta'}{2}\left|0\right\rangle\left\langle 0\right| \pm \frac{1}{4}\sin\theta\sin\theta'(\left|0\right\rangle\left\langle 1\right| + \left|1\right\rangle\left\langle 0\right|) + \sin^2\frac{\theta}{2}\cos^2\frac{\theta'}{2}\left|1\right\rangle\left\langle 1\right|\right] \otimes \left|1\right\rangle\left\langle 1\right| \\
&+ \frac{1}{2}\left[-\cos^2\frac{\theta}{2}\sin\theta'\left|0\right\rangle\left\langle 0\right| \mp \sin\theta\cos^2\frac{\theta'}{2}\left|0\right\rangle\left\langle 1\right| \mp \sin\theta\sin^2\frac{\theta'}{2}\left|1\right\rangle\left\langle 0\right| - \sin^2\frac{\theta}{2}\sin\theta'\left|1\right\rangle\left\langle 1\right|\right] \otimes \left|0\right\rangle\left\langle 1\right| \\
&+ \frac{1}{2}\left[-\cos^2\frac{\theta}{2}\sin\theta'\left|0\right\rangle\left\langle 0\right| \mp \sin\theta\sin^2\frac{\theta'}{2}\left|0\right\rangle\left\langle 1\right| \mp \sin\theta\cos^2\frac{\theta'}{2}\left|1\right\rangle\left\langle 0\right| - \sin^2\frac{\theta}{2}\sin\theta'\left|1\right\rangle\left\langle 1\right|\right] \otimes \left|1\right\rangle\left\langle 0\right|. \qquad (105)
\end{aligned}
$$

Therefore we get

$$
\begin{aligned}
\Psi &= \frac{1}{2}\left(\varphi_1 + \varphi_2\right) \\
&= \left[\cos^2\frac{\theta}{2}\cos^2\frac{\theta'}{2}\left|0\right\rangle\left\langle 0\right| \pm \frac{1}{4}\sin\theta\sin\theta'(\left|0\right\rangle\left\langle 1\right| + \left|1\right\rangle\left\langle 0\right|) + \sin^2\frac{\theta}{2}\sin^2\frac{\theta'}{2}\left|1\right\rangle\left\langle 1\right|\right] \otimes \left|0\right\rangle\left\langle 0\right| \\
&+ \left[\cos^2\frac{\theta}{2}\sin^2\frac{\theta'}{2}\left|0\right\rangle\left\langle 0\right| \pm \frac{1}{4}\sin\theta\sin\theta'(\left|0\right\rangle\left\langle 1\right| + \left|1\right\rangle\left\langle 0\right|) + \sin^2\frac{\theta}{2}\cos^2\frac{\theta'}{2}\left|1\right\rangle\left\langle 1\right|\right] \otimes \left|1\right\rangle\left\langle 1\right| \qquad (106) \\
&= \frac{1}{4}\left[(1+\cos\theta)(1+\cos\theta')\left|0\right\rangle\left\langle 0\right| \pm \sin\theta\sin\theta'(\left|0\right\rangle\left\langle 1\right| + \left|1\right\rangle\left\langle 0\right|) + (1-\cos\theta)(1-\cos\theta')\left|1\right\rangle\left\langle 1\right|\right] \otimes \left|0\right\rangle\left\langle 0\right| \\
&+ \frac{1}{4}\left[(1+\cos\theta)(1-\cos\theta')\left|0\right\rangle\left\langle 0\right| \pm \sin\theta\sin\theta'(\left|0\right\rangle\left\langle 1\right| + \left|1\right\rangle\left\langle 0\right|) + (1-\cos\theta)(1+\cos\theta')\left|1\right\rangle\left\langle 1\right|\right] \otimes \left|1\right\rangle\left\langle 1\right|. \qquad (107)
\end{aligned}
$$

Now let us define two new angles $\theta_0^{\boxast}, \theta_1^{\boxast}$ as

$$
\cos\theta_0^{\boxast} := \frac{\cos\theta + \cos\theta'}{1 + \cos\theta\cos\theta'}, \quad \cos\theta_1^{\boxast} := \frac{\cos\theta - \cos\theta'}{1 - \cos\theta\cos\theta'}. \qquad (108)
$$

Note that these are the two possible overlaps after applying the check node unitary operation.

This gives us the following identities:

$$
\begin{aligned}
\cos\frac{\theta_0^{\boxast}}{2} &= \sqrt{\frac{1}{2}(1+\cos\theta_0^{\boxast})} = \sqrt{\frac{1}{2}\frac{(1+\cos\theta)(1+\cos\theta')}{1+\cos\theta\cos\theta'}}; \quad \cos\frac{\theta_1^{\boxast}}{2} = \sqrt{\frac{1}{2}\frac{(1+\cos\theta)(1-\cos\theta')}{1-\cos\theta\cos\theta'}} \\
\sin\frac{\theta_0^{\boxast}}{2} &= \sqrt{\frac{1}{2}(1-\cos\theta_0^{\boxast})} = \sqrt{\frac{1}{2}\frac{(1-\cos\theta)(1-\cos\theta')}{1+\cos\theta\cos\theta'}}; \quad \sin\frac{\theta_1^{\boxast}}{2} = \sqrt{\frac{1}{2}\frac{(1-\cos\theta)(1+\cos\theta')}{1-\cos\theta\cos\theta'}} \\
\cos\frac{\theta_0^{\boxast}}{2}\sin\frac{\theta_0^{\boxast}}{2} &= \frac{1}{2}\frac{\sin\theta\sin\theta'}{(1+\cos\theta\cos\theta')}; \quad \cos\frac{\theta_1^{\boxast}}{2}\sin\frac{\theta_1^{\boxast}}{2} = \frac{1}{2}\frac{\sin\theta\sin\theta'}{(1-\cos\theta\cos\theta')} \qquad (109)
\end{aligned}
$$

Using these new angles and their identities in (107) we get

$$
\begin{aligned}
\Psi &= \frac{1}{2}(1+\cos\theta\cos\theta')\left[\cos^2\frac{\theta_0^{\boxast}}{2}\left|0\right\rangle\left\langle 0\right| \pm \cos\frac{\theta_0^{\boxast}}{2}\sin\frac{\theta_0^{\boxast}}{2}(\left|0\right\rangle\left\langle 1\right| + \left|1\right\rangle\left\langle 0\right|) + \sin^2\frac{\theta_0^{\boxast}}{2}\left|1\right\rangle\left\langle 1\right|\right] \otimes \left|0\right\rangle\left\langle 0\right| \\
&+ \frac{1}{2}(1-\cos\theta\cos\theta')\left[\cos^2\frac{\theta_1^{\boxast}}{2}\left|0\right\rangle\left\langle 0\right| \pm \cos\frac{\theta_1^{\boxast}}{2}\sin\frac{\theta_1^{\boxast}}{2}(\left|0\right\rangle\left\langle 1\right| + \left|1\right\rangle\left\langle 0\right|) + \sin^2\frac{\theta_1^{\boxast}}{2}\left|1\right\rangle\left\langle 1\right|\right] \otimes \left|1\right\rangle\left\langle 1\right| \qquad (110) \\
&= p_0\left|\pm\theta_0^{\boxast}\right\rangle\left\langle\pm\theta_0^{\boxast}\right| \otimes \left|0\right\rangle\left\langle 0\right| + p_1\left|\pm\theta_1^{\boxast}\right\rangle\left\langle\pm\theta_1^{\boxast}\right| \otimes \left|1\right\rangle\left\langle 1\right| \qquad (111) \\
\Rightarrow \Psi &= \sum_{j\in\{0,1\}} p_j\left|\pm\theta_j^{\boxast}\right\rangle\left\langle\pm\theta_j^{\boxast}\right| \otimes \left|j\right\rangle\left\langle j\right|, \qquad (112)
\end{aligned}
$$

where $p_0 := \frac{1}{2}(1+\cos\theta\cos\theta'), p_1 := 1 - p_0 = \frac{1}{2}(1-\cos\theta\cos\theta')$ and $\left|\pm\theta_j^{\boxast}\right\rangle := \cos\frac{\theta_j^{\boxast}}{2}\left|0\right\rangle \pm \sin\frac{\theta_j^{\boxast}}{2}\left|1\right\rangle$ for $j = 0, 1$. This

is what we desired to get initially in (91).


[1] Richardson, T. J. & Urbanke, R. L. *Modern Coding Theory* (Cambridge University Press, New York, NY, 2008).

[2] Renes, J. M. Belief propagation decoding of quantum channels by passing quantum messages. *New J. Phys.* **19**, 072001 (2017). URL `http://arxiv.org/abs/1607.04833`.

[3] Wilde, M. M. *Quantum Information Theory* (Cambridge University Press, 2013).

[4] Wilde, M. M. & Guha, S. Polar Codes for Classical-Quantum Channels. *IEEE Trans. Inform. Theory* **59**, 1175–1187 (2013). URL `https://arxiv.org/abs/1109.2591`.

[5] Guha, S. & Wilde, M. M. Polar coding to achieve the Holevo capacity of a pure-loss optical channel. In *Proc. IEEE Int. Symp. Inform. Theory*, 546–550 (2012). URL `https://arxiv.org/abs/1202.0533`.

[6] Guha, S. Structured optical receivers to attain superadditive capacity and the holevo limit. *Phys. Rev. Lett.* **106**, 240502 (2011).

[7] Helstrom, C. W. Quantum detection and estimation theory. *J. Stat. Phys.* **1**, 231–252 (1969).

[8] Helstrom, C. W., Liu, J. W. & Gordon, J. P. Quantum-mechanical communication theory. *Proc. of the IEEE* **58**, 1578–1598 (1970).

[9] Nielsen, M. A. & Chuang, I. L. *Quantum Computation and Quantum Information* (Cambridge University Press, 2010).
